# Supplementary material for: Real-time Simultaneous Multi-Object 3D Shape Reconstruction, 6DoF Pose Estimation and Dense Grasp Prediction
Source: arXiv:2305.09510 source file (2023-05-16)
Supplement: Supplementary file 1 [file appendix.tex]

\section*{APPENDIX}

Appendixes should appear before the acknowledgment.
